# Supplementary material for: The projected dynamic linear model for time series on the sphere
Source: arXiv:2308.14996 source file (2024-08-04)
Supplement: Supplementary file 1 [file appendix_convergence.tex]

\section{Convergence diagnostics for Algorithm~\ref{alg:gibbs_sampler}}
\label{app:convergence}
